# Supplementary material for: Influence-Balanced Loss for Imbalanced Visual Classification
Source: arXiv:2110.02444 source file (2021-10-06)
Supplement: Supplementary file 1 [file 7-supplementary.tex]

We thank the reviewers for their insightful comments.
% Before answering the individual reviews, we would like to point out the biggest difference between our method and the existing works.
% We believe this can help reviewers clearly understand our contribution to the research field, and provide answers to some of the raised problems. 

\textbf{Key differences from the existing methods preventing overfitting [RV \#1] :}
To the best of our knowledge, we are the first to study to improve the model after overfitting has occurred, posing a new problem setting.
In order to successfully deal with a problem, it is both important to prevent the problem beforehand and to treat it successfully after it occurs.
In terms of solving overfitting, the existing methods have been the former preventive method, while our method is the latter treatment one.
In sum, the key difference is that while other methods train a model from scratch trying to prevent overfitting, our method aims to improve the generalization performance from the already overfitted model with severe performance degradation (see Sec. 4.2.). 
Preventing overfitting during training has been studied for a long time in the machine learning community.
However, it has been rarely studied how to improve the generalization performance from the already overfitted model. 
% 오버피팅을 미리 예방하는 연구 외에, 오버피팅이 일어난 모델에 대해서 성능을 개선하는 것은 머신러닝 커뮤니티에서 지금까지 무시되었던 중요한 문제가 될 수 있다.
This could be a very important issue in practice.
For example, in practice, it is difficult to know if there exist noisy labels in advance.
Thus, it is common to train the model first, under the assumption that the collected dataset is clean.
Especially when it takes a lot of time to train the model, it would be more beneficial to improve the model, than training again from scratch.
In addition, since our method does not require specially-designed architecture or training scheme, it can be easily used in combination with other methods.
Regarding this, thank you for the additional references. We will add these references, and discuss the key differences in the paper.

\textbf{Computational Efficiency of Hessian [RV \#1, \#4]:} 
We understand your points, but we can alleviate this issue. First, we only calculate the last FC layer, which reduces the dimension of the matrix a lot. Also, thanks to the active studies in optimization theory, the methods for efficiently calculating the inverse of the Hessian matrix have been proposed (please see our Supplementary Material).

% Moreover, parallel computing can be helpful when computing the criteria for N training points. For example, since only 1GB memory is required to calculate the overfitting score on data (CIFAR-10 setting), we splitted training points into three chunks and ran the code simultaneously. This naive modification cut the training time in half. 

\textbf{How to distinguish hard examples (Outliers) [RV \#1, \#3]:} 
As you pointed, it might be possible that some correctly-labeled hard examples could be also removed.
However, we wonder if we can say that the correctly-labeled hardly-fit data (outliers) would be helpful for training a robust model. 
If the correctly-labeled data plays as an outlier (hardly to fit), fitting on that data may lead a model to form an overfitted decision boundary.
Not to damage the model performance due to underfitting, we use some removed data with newly corrected labels (Lines 227-234).

 %(Weak Reject) 
\textbf{Additional clean validation set [RV \#3, \#4]:} It is common to use a small number of additional clean validation set in the literature. 
While [Song et al., ICML'20, NguYen et al., ICLR'20] used 1,000 clean validation samples, and [Jiang et al., ICML'18] used 5,000 clean validation samples, we used only 500 samples.

\textbf{Fair experimental comparison to other works [RV \#3, \#5]:}
Comparison on equal setting is a problem for all papers in this area, and we try to be fair.
Unfortunately, it is impossible to compare our method with other studies on the exact same setting.
It is because, as discussed in the first paragraph about key differences, our method aims to improve the overfitted model suffering from severe performance degradation.
On contrary, no other methods start training from the overfitted model, because they aim to utilize small losses before the model overfits to the noisy labels.  
Thus, it would be fair comparison if we compare the improvement of other methods from the overfitted model. 
However, to show where our performance can be positioned, we compared our method with other state-of-the-art methods.
In addition, we compared with the same architecture (ResNet-34), except that the results reported from [Huang et al.,] used ResNet-101. 
% In addition, since the random seed used for data generation in the other papers is not known, we compared with their reported performances.

% 이와 관련하여 따라서 완전히 똑같은 상황에서 다른 연구와 비교하는 것은 불가능하다.
% Experimental Section "Effects of Iterative Removing and Retraining" 에서 언급했듯, 우리는 모델을 처음부터 트레이닝한 것이 아니고, CIFAR-10 에 대해 각각 accuracy가 88.15\%, 70.18\%, 46.64\%, and 19.35\% 까지 떨어진 모델로부터 성능 개선을 시작했기 때문이다. 
% 반면, 다른 논문들은 모델 accuracy가 저렇게 심하게 degradation 된 상태에서 시작하지 않는다. 
% 이 때문에 비교가 불가능하다고 볼 수 있지만, 우리 메서드의 결과가 어느정도 위치에 있는지 알려주기 위해 다른 sota method와 비교하였다.
% 가능한 fair한 비교를 위해 우리는 ResNet-34 를 사용하고 같은 noise label에 대해서 비교하였고, 다른 논문에서 데이터 생성에 사용한 random seed를 알지 못하기 때문에 그들이 레포트한 결과가 가장 좋을 것으로 가정하고 해당 논문에서 리포트한 best accuracy를 비교하였다. 

\textbf{Tuning hyper-parameters [RV \#4, \#5]:}
We agree that setting hyper-parameters may require additional tuning work.
First, $\alpha$ can be simply set to 0, because our method targets influential samples. 
Also, to provide a common rule, we experimented with various $\beta$ and $\gamma$, and included the best strategy and discussion in Supplementary Material.
Meanwhile, since $\beta$ and $\gamma$ are used to decide the number of training samples to remove, a prior knowledge about noise rates can be utilized if it exists in practice.
We leave this to the future work that can identify optimal hyper-parameters that can be dynamically adjusted in iterations.

add (minor points)
